# Supplementary material for: Cryptography Is Not Enough: Relay Attacks on Authenticated GNSS Signals
Source: arXiv:2204.11641 source file (2022-11-02)
Supplement: Supplementary file 1 [file appendix.tex]

% \begin{figure} [t]
% \centerline{\includegraphics[width=3.2in]{figures/gnuradio2.png}}
% \caption{A GNURadio flowgraph showing the implementation of our Spoofing Signal Synthesizer. The file source provides samples for individual satellite signals. Next, the delay block adds appropriate delays. Finally, the delayed signals are combined and dumped through a file sink for further processing.}
% \label{gnuradio}
% \end{figure}

% \begin{figure} [t]
% \centerline{\includegraphics[width=3.2in]{figures/implementation.pdf}}
% \caption{A flowgraph showing the implementation of our attack in real-time}
% \label{implementation_flowgraph}
% \end{figure}
